# Supplementary material for: Sector Models - A Toolkit for Teaching General Relativity. Part 1: Curved Spaces and Spacetimes
Source: arXiv:1405.0323 ancillary file (2014-07-06)

Sector Model "Black Hole"  
Sektormodell "Schwarzes Loch"

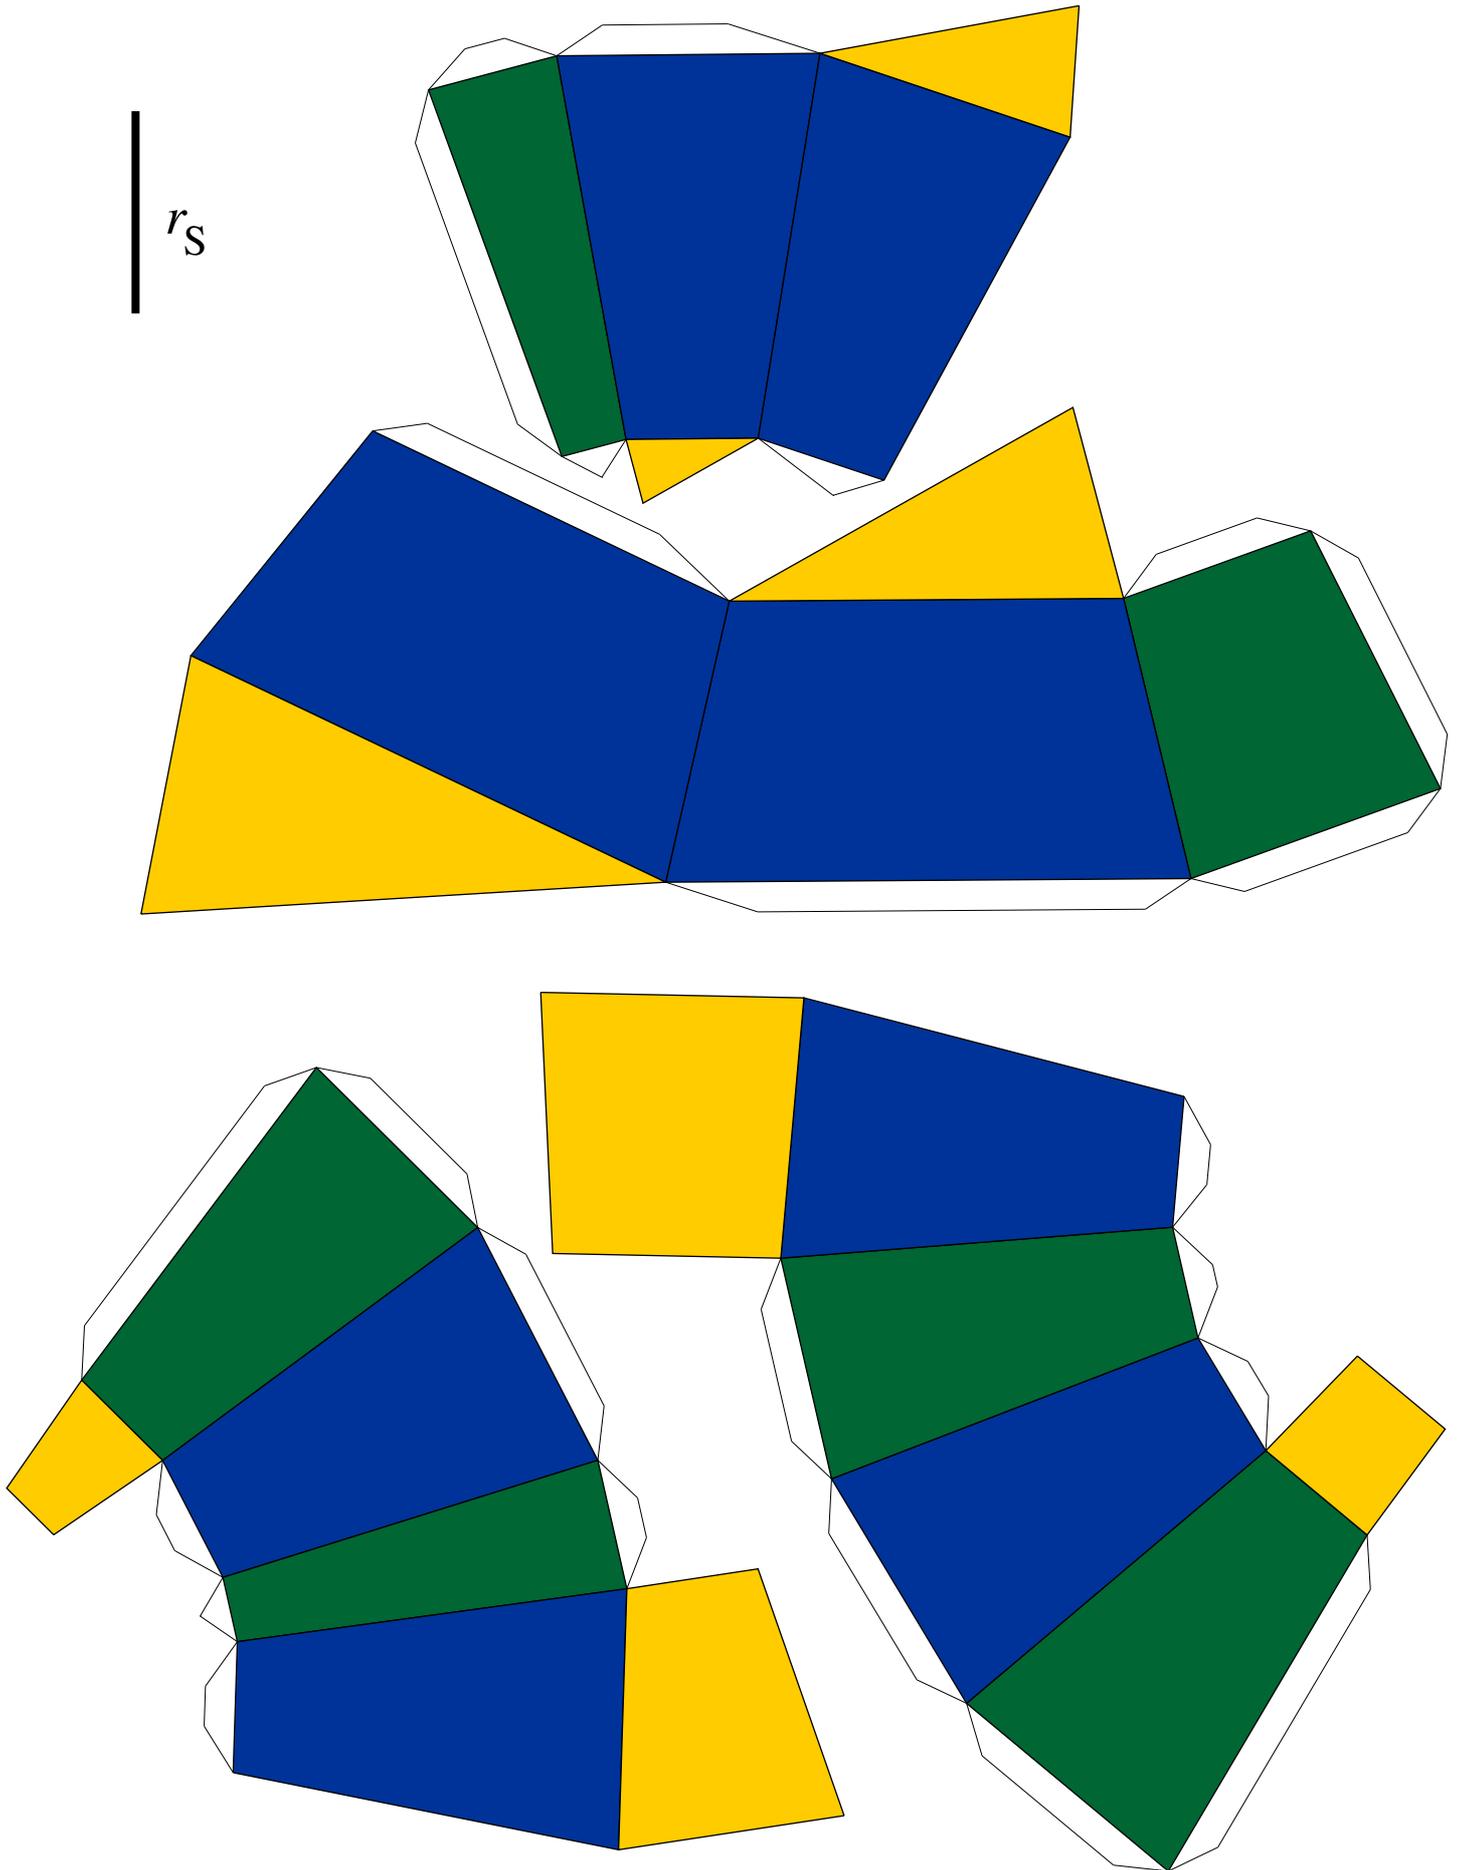

Sector Model "Black Hole"  
Sektormodell "Schwarzes Loch"

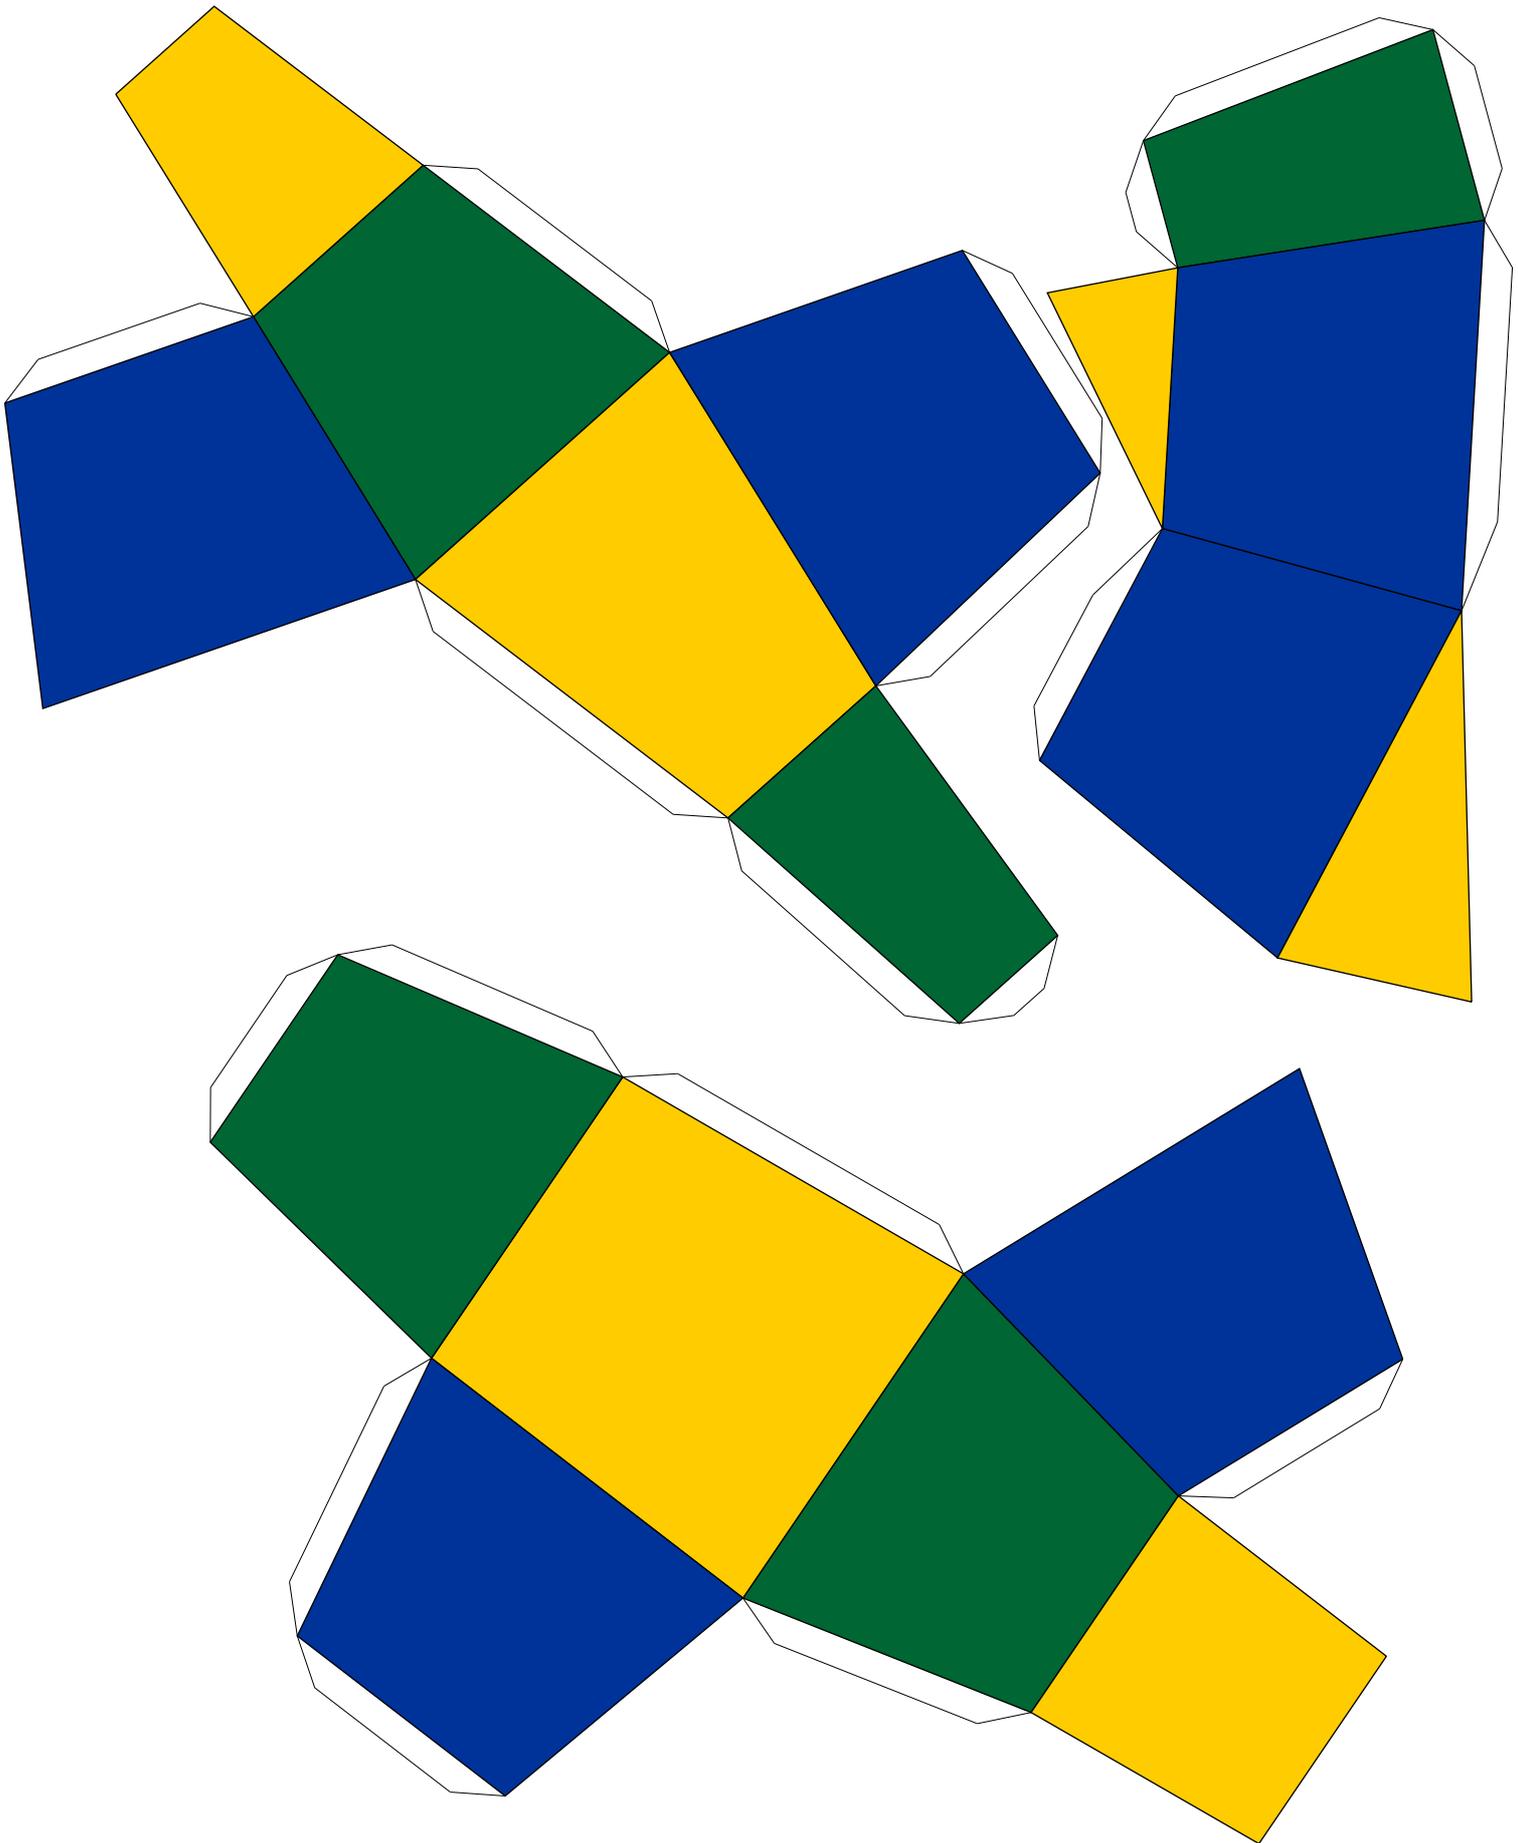

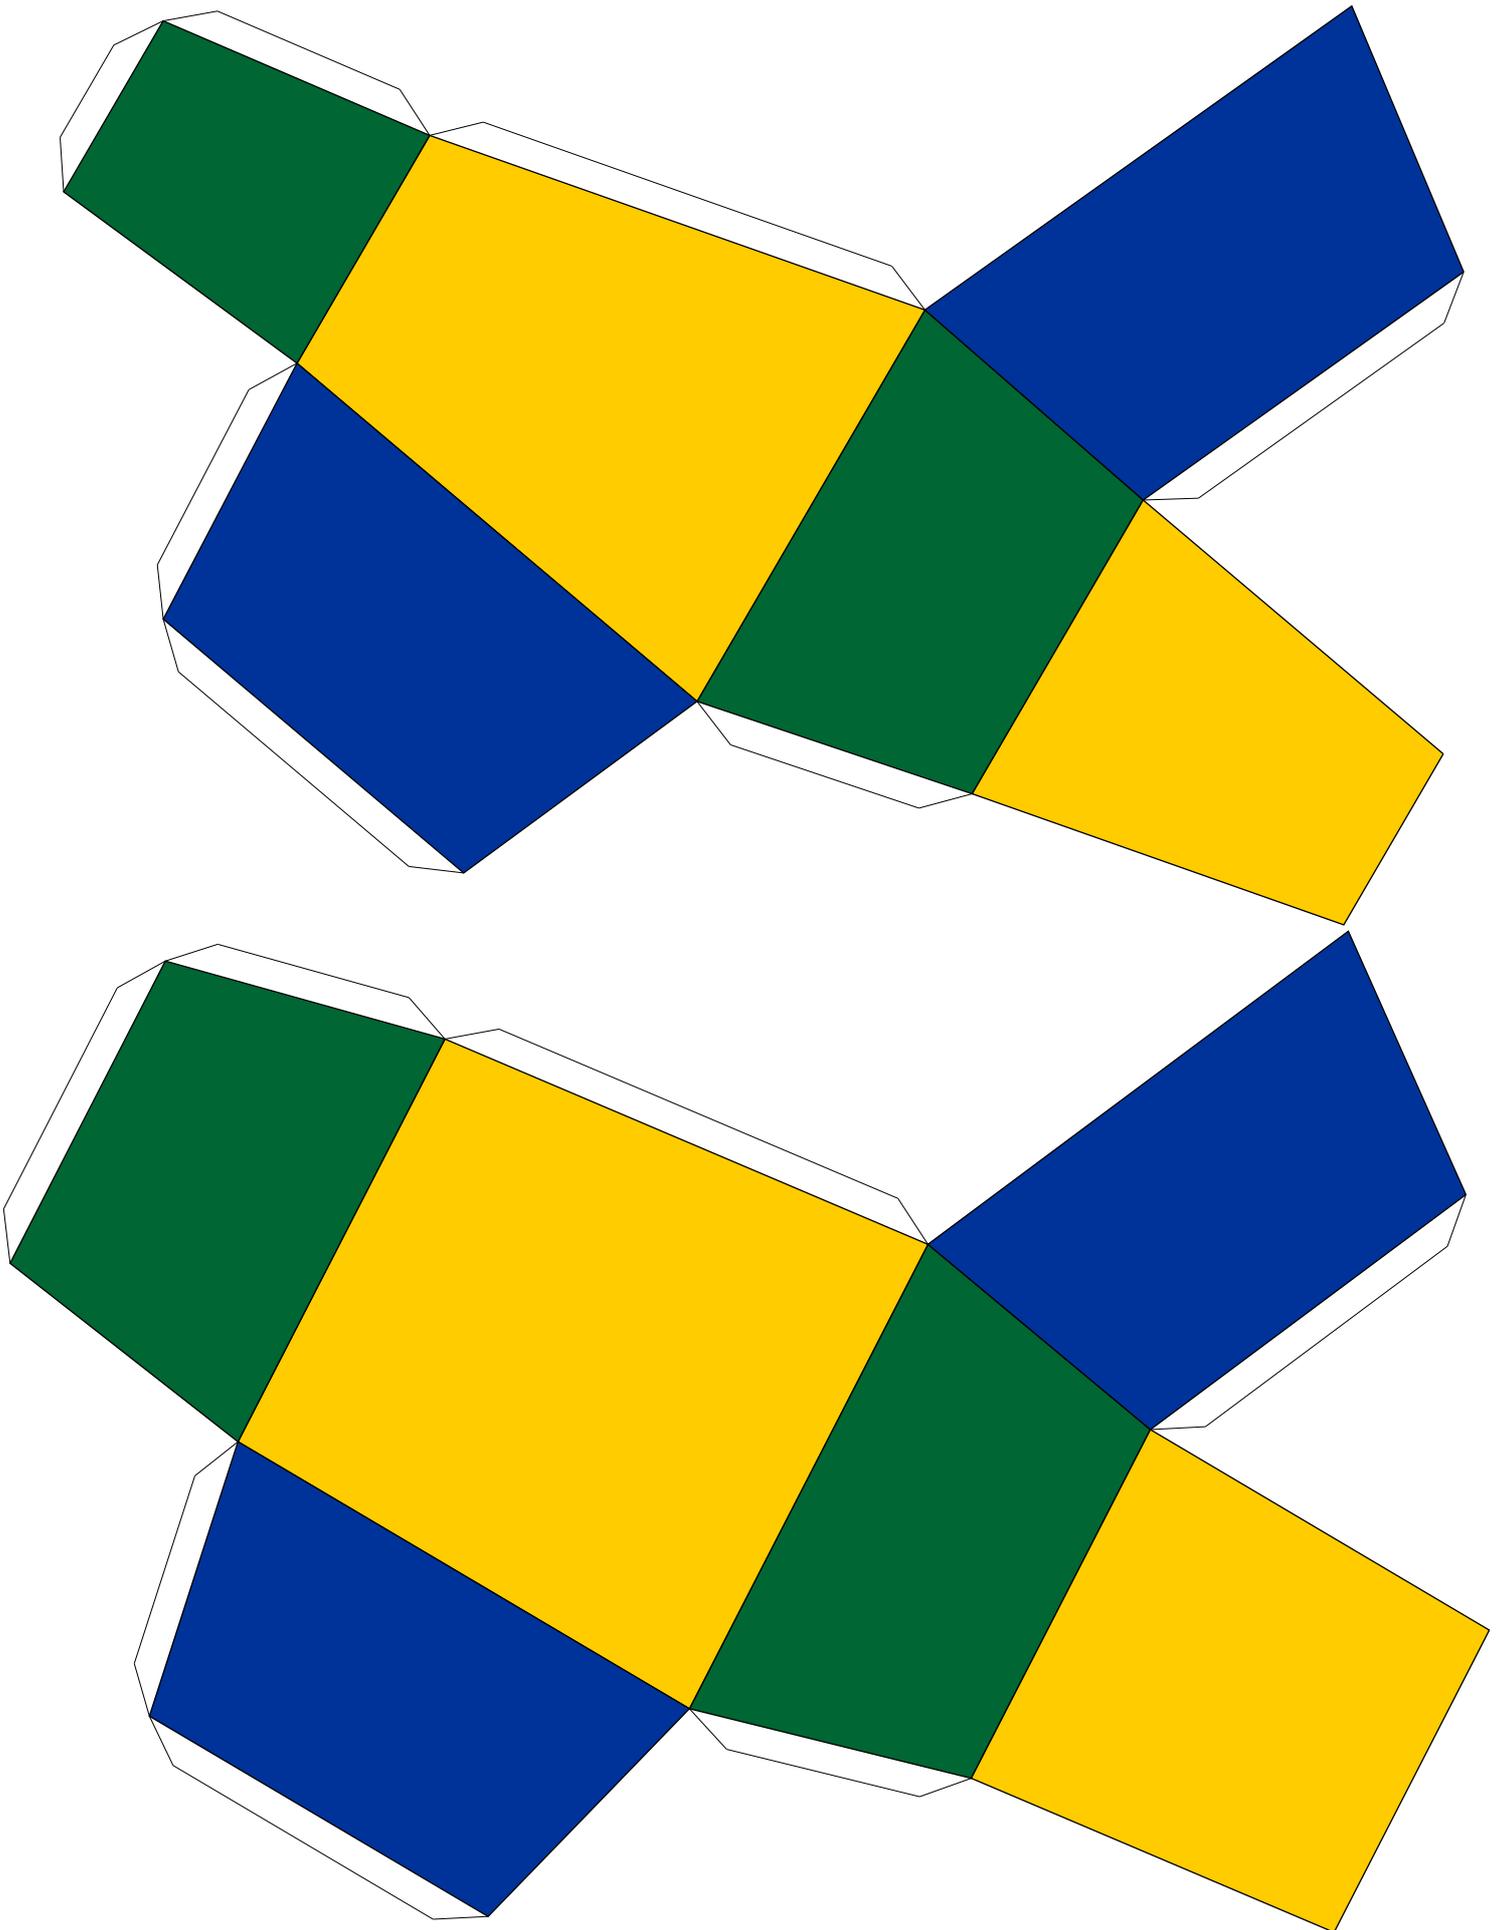

Supplement: Supplementary file 1 [file black_hole.pdf]
