# Supplementary material for: Sector Models - A Toolkit for Teaching General Relativity. Part 1: Curved Spaces and Spacetimes
Source: arXiv:1405.0323 ancillary file (2014-07-06)

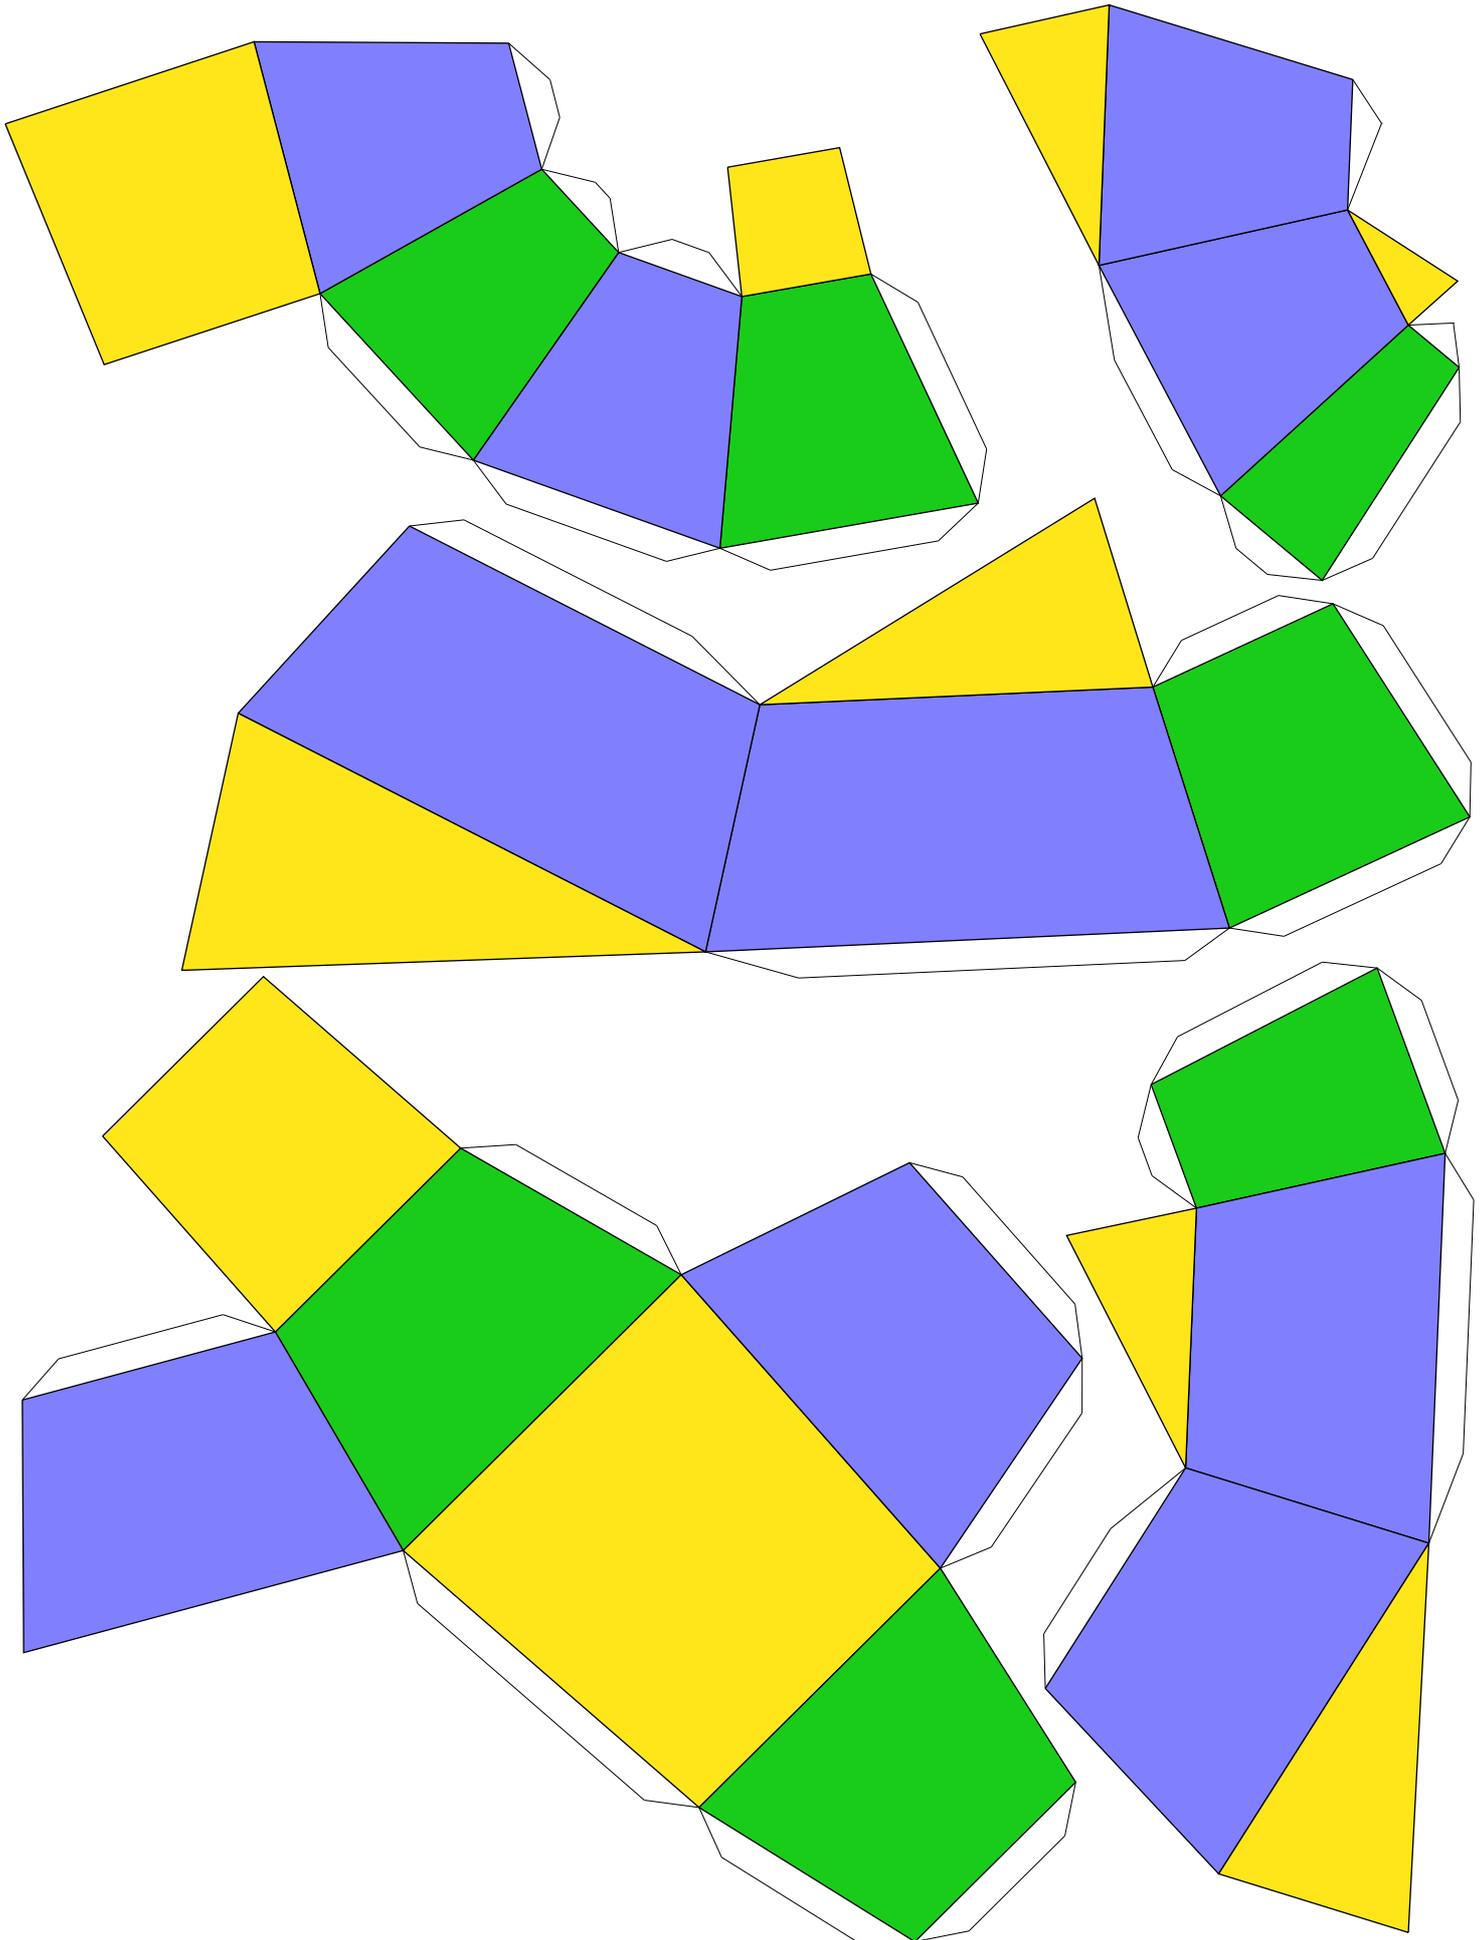

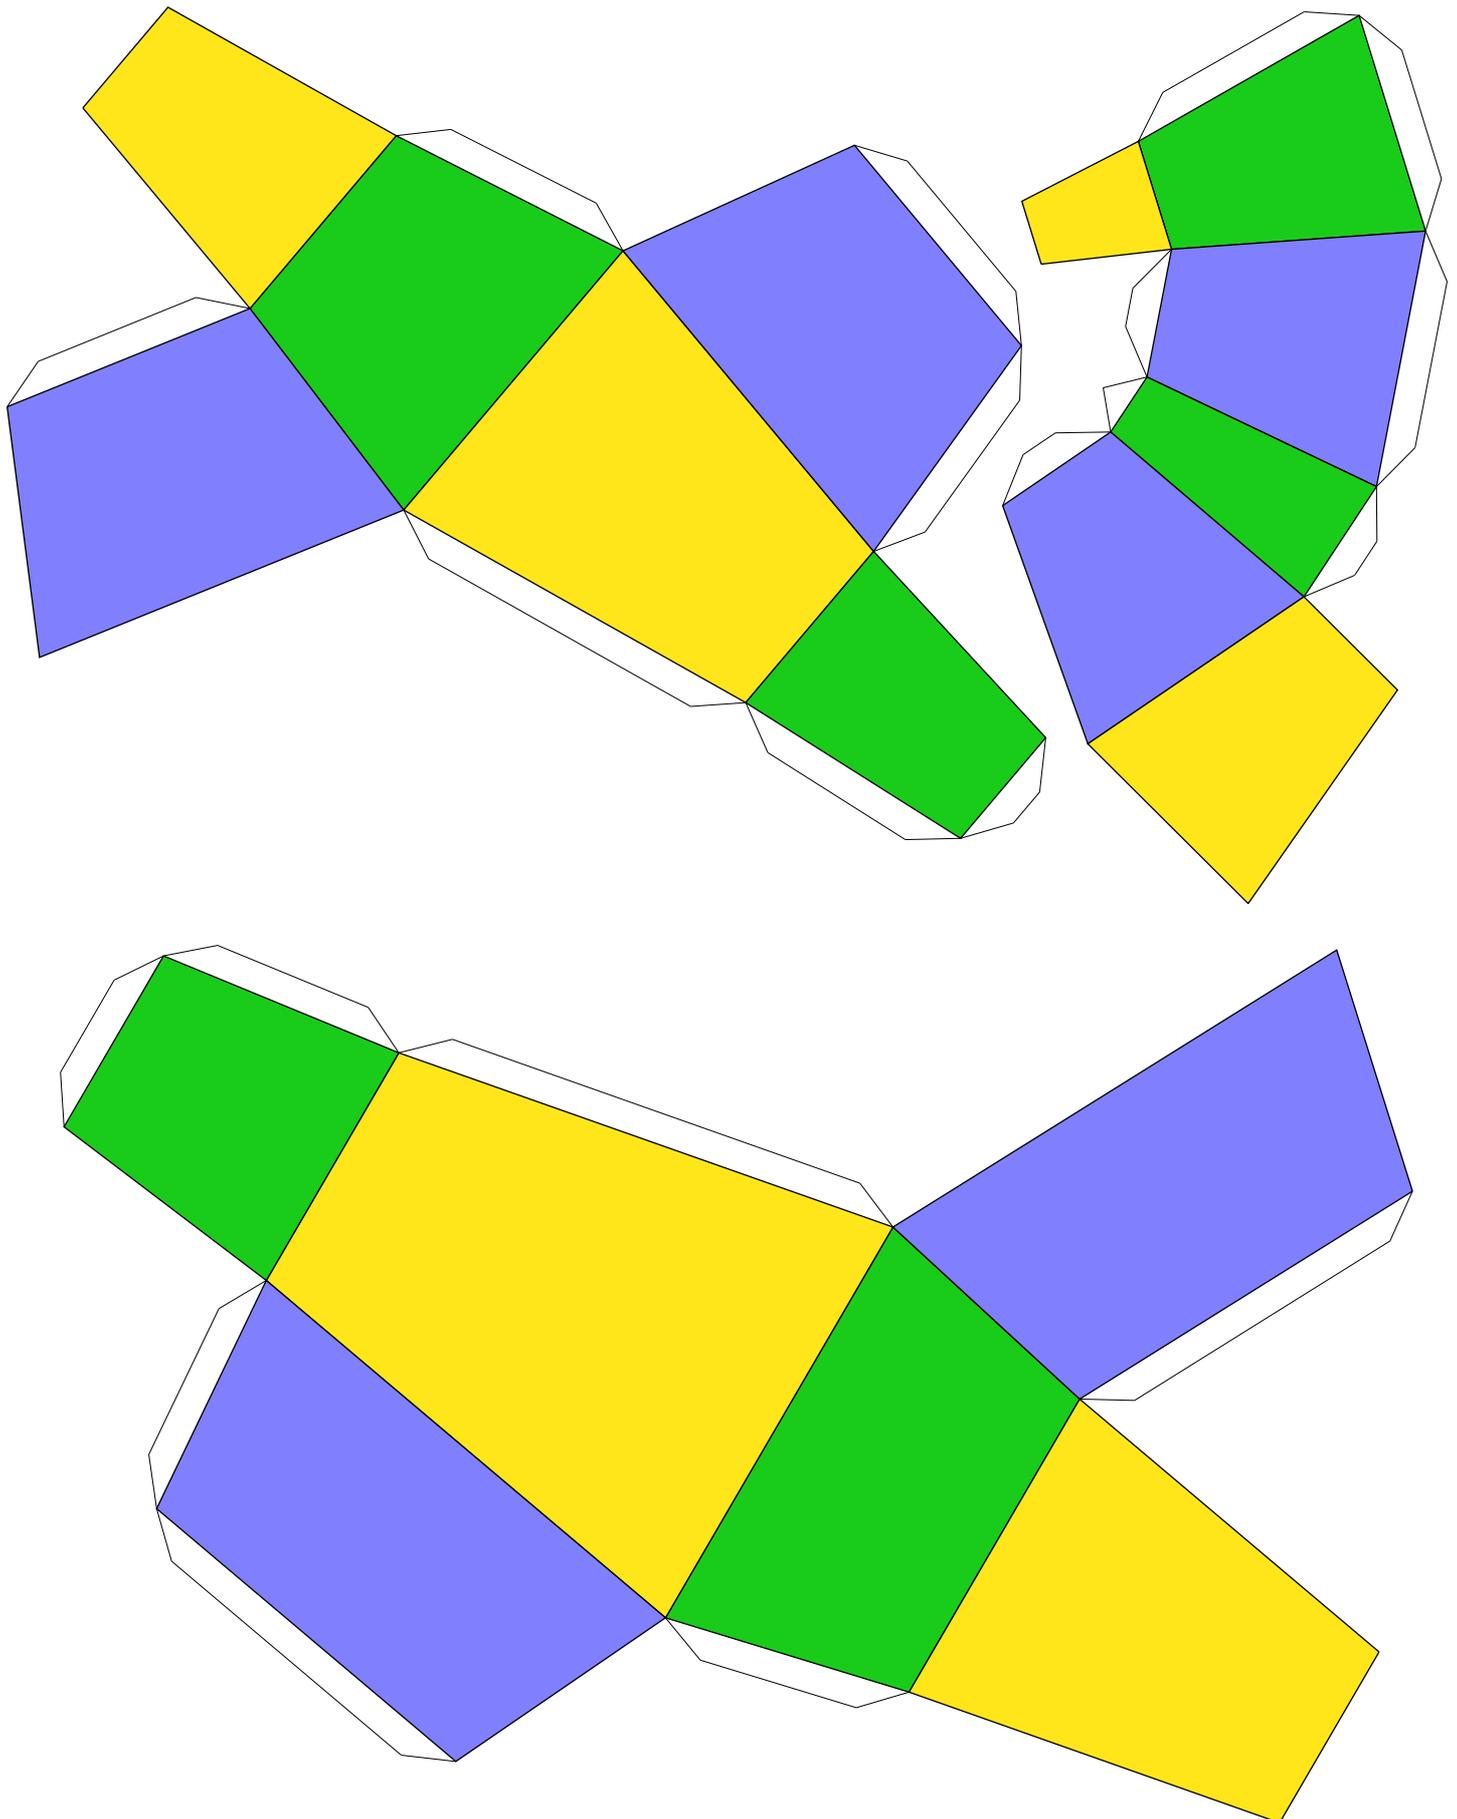

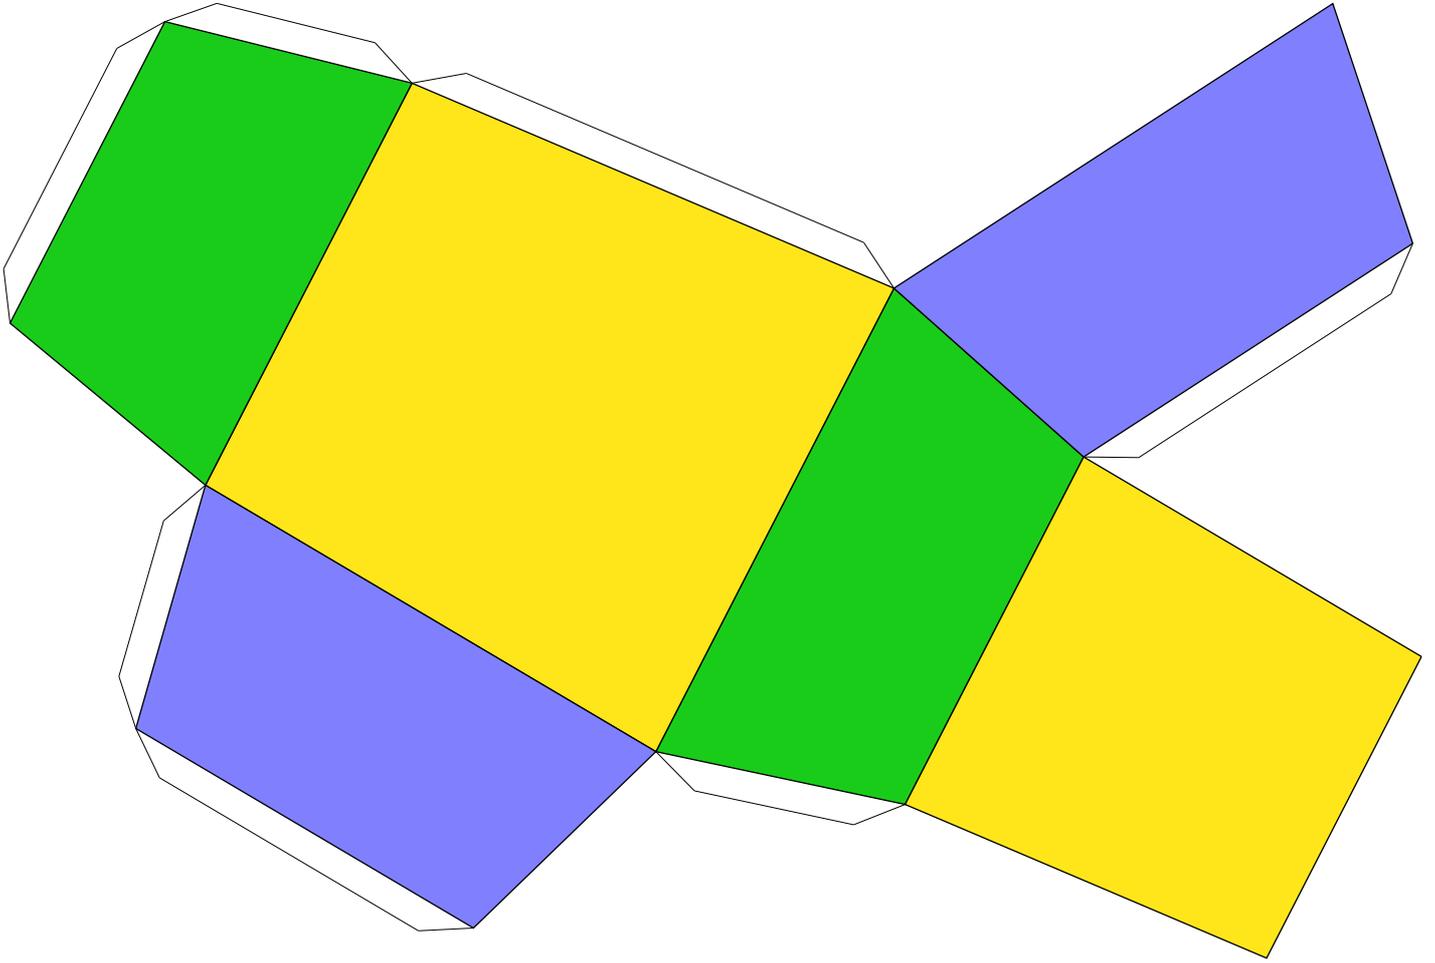

Supplement: Supplementary file 2 [file euclidean_space.pdf]
